# Supplementary material for: Border effect corrections for diagonal line based recurrence quantification analysis measures
Source: arXiv:1909.09211 source file (2019-09-19)
Supplement: Supplementary file 1 [file fig_appendix_results_5.pdf]

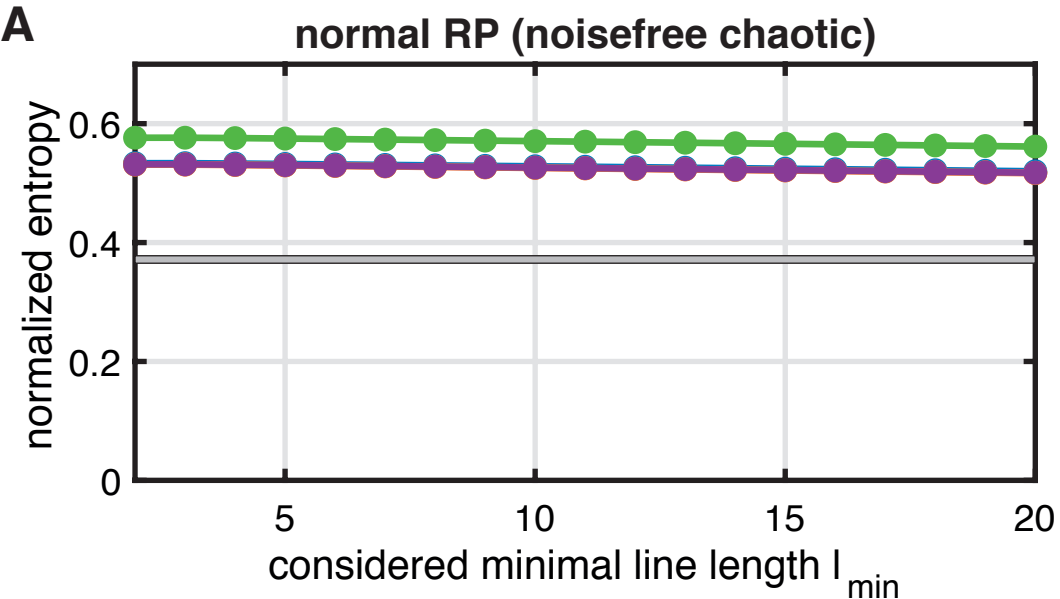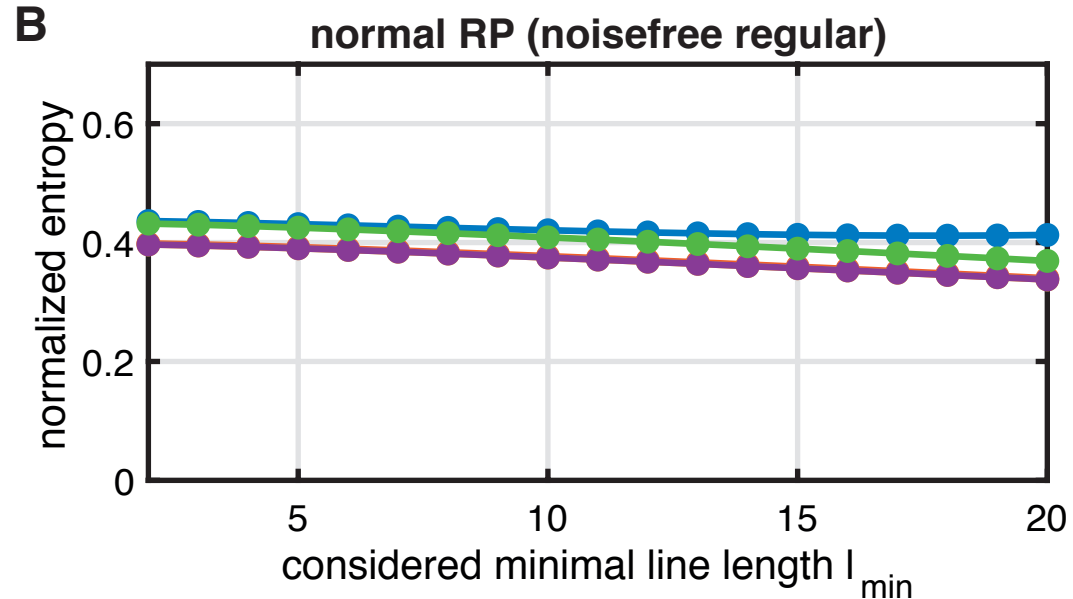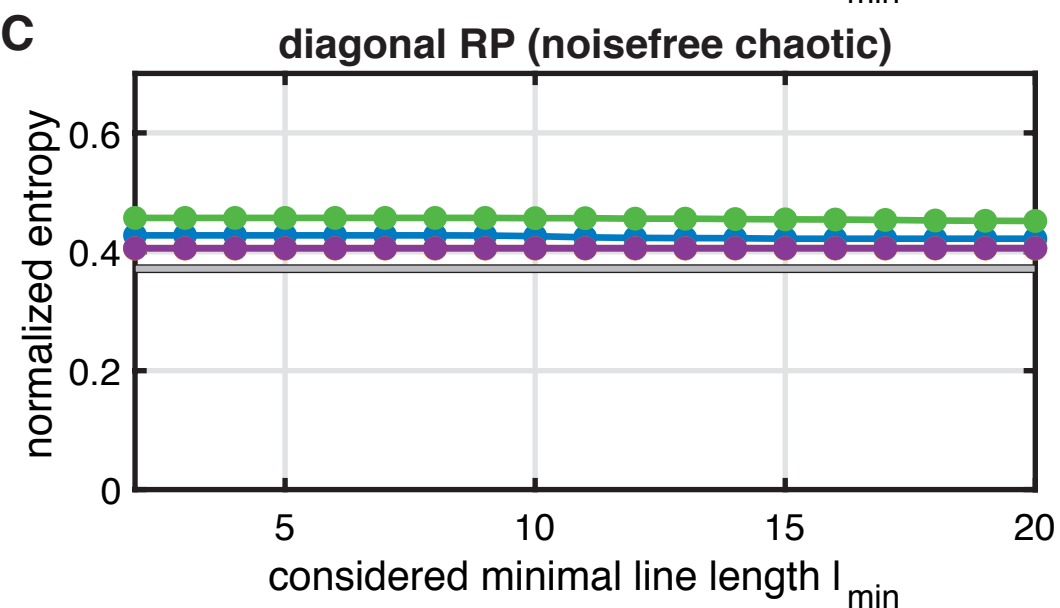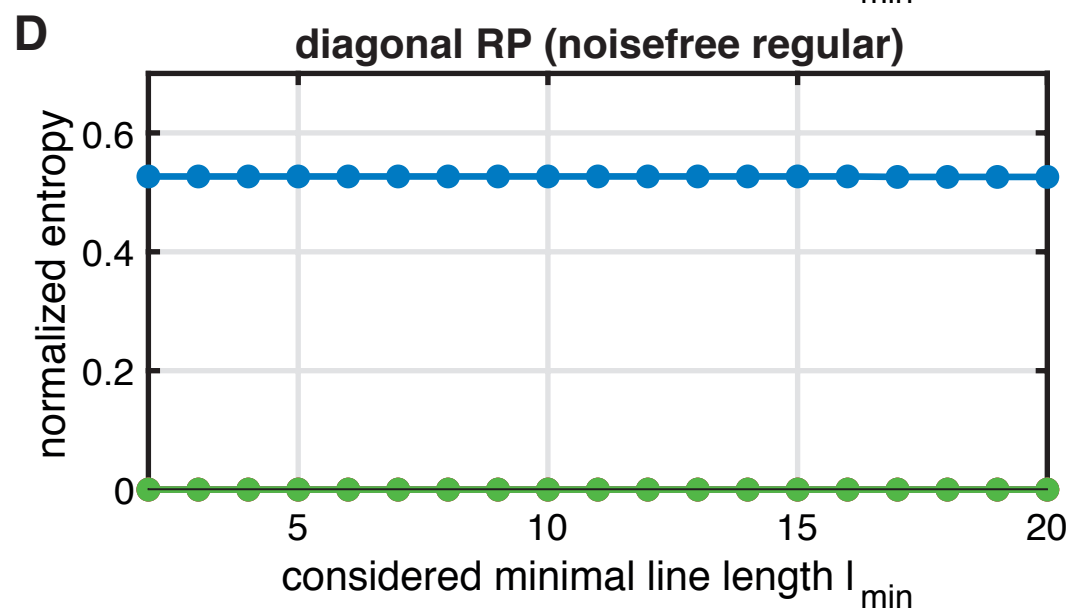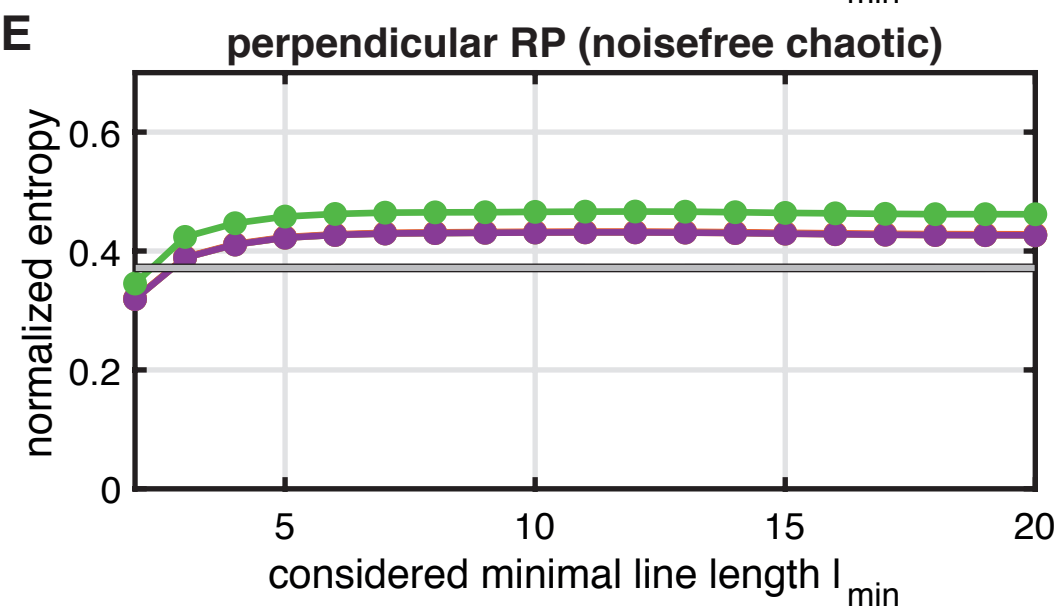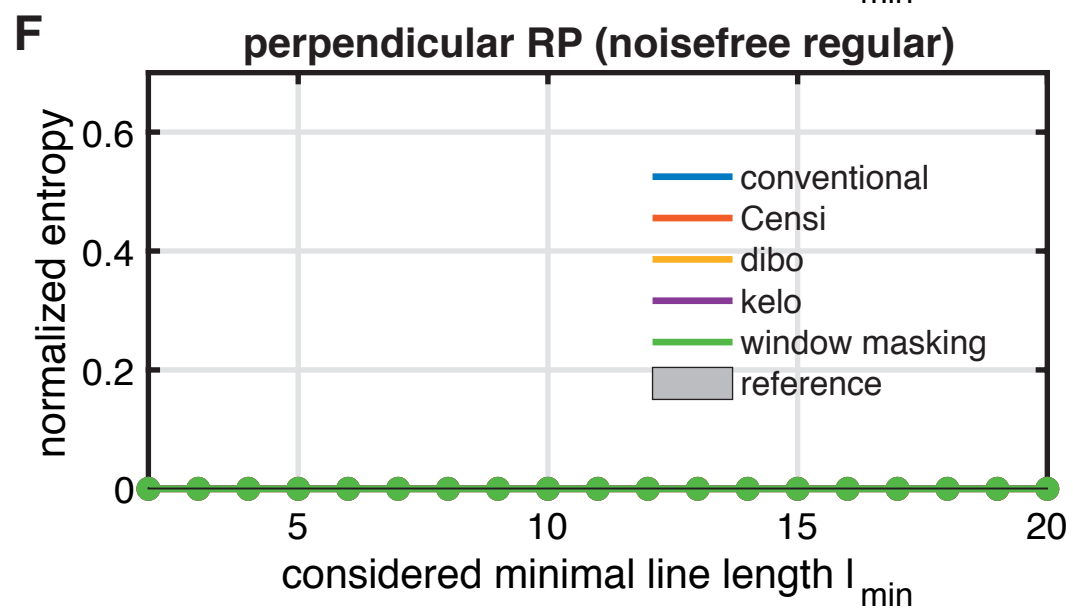

normal RP (noise free regular)
